# Supplementary material for: Constrained Correlated Equilibria
Source: arXiv:2309.05218 source file (2023-09-12)
Supplement: Supplementary file 2 [file Preliminaries.tex]

\begin{proposition}
        Let $G$ be a finite non-cooperative game and $d= (\Omega, (\mathcal{P}_i)_{i\in\mathcal{N}}, \bm{q})$ a correlation device. The strategy $\bm{\alpha}^* = (\alpha_i^*)_{i \in \mathcal{N}} : \Omega \rightarrow \mathcal{A}$ is a correlated equilibrium if and only if
    \begin{equation}
        \sum_{\omega \in \Omega} \bm{q}(\omega) \left[u_{i}({\alpha}_i^*(\omega), \bm{\alpha}_{-i}^*(\omega)) - u_{i}(\tau^\prime_i(\omega), \bm{\alpha}^*_{-i}(\omega))\right] \geq 0
    \end{equation}
    for every player $i$ and every $\tau_i^\prime$ function of $\alpha^*_i$.
\end{proposition}
%%%%%%%%%%%%%%%%%%%%%%%%%%
%%%%%%%%%%%%%%%%%%%%%%%%%%
\begin{proof}
Suppose $\bm{\alpha}^*= (\alpha^*_i)_{i \in \mathcal{N}}$ is an $n$-tuple of correlated strategies with $\alpha_i^* : \Omega \rightarrow \mathcal{A}_i$ satisfying
%%%%%%%%%%%%%%%%%%%
\begin{align}
    \sum_{\omega \in \Omega} \bm{q}(\omega) \left[u_{i}({\alpha}_i^*(\omega),\bm{\alpha}_{-i}^*(\omega)) - u_{i}(\tau^\prime_i(\omega), \bm{\alpha}^*_{-i}(\omega))\right] \geq 0 \label{eq:defn1}
\end{align}
%%%%%%%%%%%%%%%%%%%
for each player $i$ and each $\tau^\prime_i$ function of $\alpha_i^*$. The function $\tau_i^\prime$ that are function of $\alpha_i^*$ are in the set:
%%%%%%%%%%%%%%%%%%%
\begin{align}
    \Theta_{\alpha_i^*} = \{ \alpha^\prime_i : \Omega \rightarrow \mathcal{A}_i \text{ s.t } \exists h_i : {\mathcal{A}_i} \rightarrow {\mathcal{A}_i} \mid  \alpha^\prime_i = h_i \circ \alpha_i^* \}
\end{align}
%%%%%%%%%%%%%%%%%%%
Hence, we can re-write the conditions in Eq. (\ref{eq:defn1}) satisfied by $\bm{\alpha}^*$ as follows:
%%%%%%%%%%%%%%%%%%%
\begin{align}
    \forall i \in \mathcal{N},
    \forall \tau_i^\prime \in \Theta_{\alpha^*_i} 
    \quad
    \sum_{\omega \in \Omega} \bm{q}(\omega) \left[u_{i}({\alpha}_i^*(\omega),\bm{\alpha}_{-i}^*(\omega)) - u_{i}(\tau^\prime_i(\omega), \bm{\alpha}^*_{-i}(\omega))\right] \geq 0
\end{align}
%%%%%%%%%%%%%%%%%%%
\noindent Now, consider the correlation device $d = (\Omega, (\mathcal{P}_i)_{i \in \mathcal{N}}, \bm{q})$ where the partition $\mathcal{P}_i$ is induced by player $i$'s equilibrium strategy $\alpha_i^*$:
%%%%%%%%%%%%%%%%%%%
\begin{align}
    \mathcal{P}_i = \{ \omega \in \Omega : \alpha_i^{*}(\omega) = a_i \}_{a_i \in \mathcal{A}_i}
\end{align}
%%%%%%%%%%%%%%%%%%%
We prove that the strategies $\tau_i^\prime$ in the set $\Theta_{{\alpha}^*_i}$ are exactly the $\mathcal{P}_i$-measurable mappings $\alpha_i^* : \Omega \rightarrow \mathcal{A}_i$ in $\mathcal{S}_{i, d}$ \ie $\mathcal{S}_{i,d} = \Theta_{\bm{\alpha}^*_i}$ for every player $i$.\\
%\textcolor{red}{Consider the $\sigma$-algebra generated by the partition $\mathcal{P}_i$ denoted by $\sigma(\mathcal{P}_i)$ consisting of all possible unions of the elements of the partition (including the empty set).}\\
By definition, the function $\tau^\prime_i: \Omega \rightarrow \mathcal{A}_i$ is measurable with respect to the $\sigma$-algebra $\sigma(\mathcal{P}_i)$ generated by the partition $\mathcal{P}_i$ if and only if $\tau_i^{\prime}$ is constant on each set element of the partition.\\
Let $P_{a_i} \in \mathcal{P}_i$ be the element of the partition such that $\forall \omega \in P_{a_i}, \alpha_i^*(\omega) = a_i$ , we have:
%%%%%%%%%%%%%%%%%%%
\begin{align}
    \forall \omega \in P_{a_i},
    \quad \tau_i^{\prime}(\omega) & = (h_i \circ \alpha_i^*)(\omega) = h_i ( \alpha_i^*(\omega)) = h_i(a_i)
\end{align}
%%%%%%%%%%%%%%%%%%%
Hence the function is constant on the element of the partition $P_{a_i}$. Therefore, the function $\tau_i^\prime$ are the $\mathcal{P}_i$-measurable functions and $\Theta_{{\alpha}^*_i} = \mathcal{S}_{i, d}$.
To conclude, the two definitions are equivalent and characterize the same set of $n$-tuples of correlated equilibrium strategies.
\begin{flushright}                                      
$\blacksquare$
\end{flushright}
\end{proof}

%\section*{Appendix B}
\newpage

\begin{proposition}
    Let $G$ be a finite non-cooperative game and $d= (\Omega, (\mathcal{P}_i)_{i\in\mathcal{N}}, \bm{q})$ a correlation device. The strategy $\bm{\alpha}^* = (\alpha_i^*)_{i \in \mathcal{N}} : \Omega \rightarrow \mathcal{A}$ is a correlated equilibrium if and only if
    \begin{align}
        & \forall i \in \mathcal{N},
        \forall a_{i} \in \mathcal{A}_{i},
        \forall \omega \in \Omega \nonumber \\
        & \sum_{\omega^{\prime} \in P_{i}(\omega)} \bm{q}(\omega^{\prime}) \left[u_{i}({\alpha}_i^*(\omega^{\prime}), \bm{\alpha}_{-i}^*(\omega^{\prime})) - u_{i}(a_i, \bm{\alpha}^*_{-i}(\omega^{\prime}))\right] \geq 0 
    \end{align}
\end{proposition}

\begin{proof}
$(\Rightarrow)$
We suppose that $\bm{\alpha}^*$ is a correlated equilibrium strategy satisfying
\begin{align}
& \forall i \in \mathcal{N},
\forall \alpha^\prime_{i} : \Omega \rightarrow \mathcal{A}_{i} \nonumber\\
& \sum\limits_{\omega^\prime \in \Omega} \bm{q}(\omega^\prime ) u_{i}({\alpha}_i^*(\omega^{\prime}),\bm{\alpha}_{-i}^*(\omega^\prime)) \geq \sum\limits_{\omega^\prime \in \Omega} \bm{q}(\omega^\prime) u_{i}(\alpha^\prime_{i}(\omega^\prime), \bm{\alpha}^*_{-i}(\omega^\prime)) \label{eq:average}
\end{align}
Let $\mathcal{P}_i = \{  P_{i, 1}, P_{i, 2}, ..., P_{i, n_i} \}$ and consider the deviation strategy $\alpha^\prime_i$ in Eq. (\ref{eq:strategy}), equal to player $i$'s equilibrium strategy $\alpha_i^*$ except on a single element of the partition
\begin{align}\label{eq:strategy}
    \alpha^\prime_i(\omega^\prime) = 
    \begin{cases}
    \alpha^*_i(\omega^\prime), & \text { if } \omega^\prime \in \Omega - \{P_{i, j}\}, \\
    a_i, & \text { otherwise. }
    \end{cases}
\end{align}
Eq. (\ref{eq:average}) can be written for any player $i \in \mathcal{N}$ and any strategy $\alpha^\prime_i$ of the form Eq. (\ref{eq:strategy})
\begin{align}
    \sum\limits_{\mathclap{\omega^\prime \in P_{i, j}}} \bm{q}(\omega^\prime ) u_{i}({\alpha}_i^*(\omega^{\prime}), \bm{\alpha}_{-i}^*(\omega^\prime)) + \sum\limits_{\mathclap{\omega^\prime \in \Omega - \{P_{i, j}\}}} \bm{q}(\omega^\prime ) u_{i}({\alpha}_i^*(\omega^{\prime}),\bm{\alpha}_{-i}^*(\omega^\prime)) \geq \nonumber \\
    \sum\limits_{\mathclap{\omega^\prime \in P_{i, j}}} \bm{q}(\omega^\prime) u_{i}(a_{i}, \bm{\alpha}^*_{-i}(\omega^\prime)) + \sum\limits_{\mathclap{\omega^\prime \in \Omega - \{P_{i, j}\}}} \bm{q}(\omega^\prime) u_{i}(\alpha_{i}^*(\omega^\prime), \bm{\alpha}^*_{-i}(\omega^\prime))
\end{align}
Hence, after simplifying the second term on both sides, we obtain
\begin{align}
    \sum\limits_{\omega^\prime \in P_{i, j}} \bm{q}(\omega^\prime ) u_{i}({\alpha}_i^*(\omega^{\prime}),\bm{\alpha}_{-i}^*(\omega^\prime)) \geq \sum\limits_{\omega^\prime \in P_{i, j}} \bm{q}(\omega^\prime) u_{i}(a_{i}, \bm{\alpha}^*_{-i}(\omega^\prime))
\end{align}
Let $\omega \in P_{i,j}$, and denote the partition the j$^{th}$ element of player $i$'s partitioning $P_{i,j}$ containing $\omega$ by $P_{i,j}= P_i(\omega)$.
We then have
\begin{align}
    & \forall i \in \mathcal{N},
    \forall a_{i} \in \mathcal{A}_i,
    \forall \omega \in \Omega \nonumber \\
    & \sum\limits_{\omega^\prime \in P_{i}(\omega)} \bm{q}(\omega^\prime ) u_{i}({\alpha}_i^*(\omega^{\prime}),\bm{\alpha}_{-i}^*(\omega^\prime)) \geq \sum\limits_{\omega^\prime \in P_{i}(\omega)} \bm{q}(\omega^\prime) u_{i}(a_{i}, \bm{\alpha}^*_{-i}(\omega^\prime))
\end{align}
$(\Leftarrow)$ We now assume that the strategy $\bm{\alpha}^*$ satisfies,
\begin{align}
    & \forall i \in \mathcal{N},
    \forall a_i \in \mathcal{A}_{i},
    \forall \omega \in \Omega \nonumber \\
    & \sum_{\omega^{\prime} \in P_{i}(\omega)} \bm{q}(\omega^{\prime}) u_{i}({\alpha}_i^*(\omega^{\prime}),\bm{\alpha}_{-i}^*(\omega^{\prime})) \geq \sum_{\omega^{\prime} \in P_{i}(\omega)} \bm{q}(\omega^{\prime}) u_{i}(a_{i}, \bm{\alpha}^*_{-i}(\omega^{\prime})) \label{eq:conditionalInequality}
\end{align}
Let $\mathcal{P}_i = \{  P_{i, 1}, P_{i, 2}, ..., P_{i, n_i} \}$.
The inequalities in Eq. (\ref{eq:conditionalInequality}) imply
\begin{align}
    & \forall i \in \mathcal{N},
    \forall a_{i} \in \mathcal{A}_i,
    \forall P_{i,j} \in \mathcal{P}_i \nonumber \\
    & \sum_{\omega^{\prime} \in P_{i,j}} \bm{q}(\omega^{\prime}) u_{i}({\alpha}_i^*(\omega^{\prime}),\bm{\alpha}_{-i}^*(\omega^{\prime})) \geq \sum_{\omega^{\prime} \in P_{i,j}} \bm{q}(\omega^{\prime}) u_{i}(a_{i}, \bm{\alpha}^*_{-i}(\omega^{\prime}))
\end{align}
Summing over all elements $P_{i,j}$ of the partition $\mathcal{P}_i$,
\begin{align}
    & \forall i \in \mathcal{N},
    \forall \alpha^\prime_{i} : \mathcal{P}_i \rightarrow \mathcal{A}_{i} \\
    & \sum_{ P_{i,j} \in \mathcal{P}_i} \sum_{\omega^{\prime} \in P_{i,j}} \bm{q}(\omega^{\prime}) u_{i}({\alpha}_i^*(\omega^{\prime}),\bm{\alpha}_{-i}^*(\omega^{\prime})) \geq \sum_{P_{i,j} \in \mathcal{P}_i} \sum_{\omega^{\prime} \in P_{i,j}} \bm{q}(\omega^{\prime}) u_{i}(\alpha^\prime_{i}(\omega^\prime), \bm{\alpha}^*_{-i}(\omega^{\prime})) \label{eq:ref} \nonumber
\end{align}
where $\alpha^\prime_i$ is a function mapping each element $P_{i,j}$ of $\mathcal{P}_i$ to an action $a_i \in \mathcal{A}_i$.
Since for every player the set $\mathcal{P}_i$ is a partition of $\Omega$, Eq. (\ref{eq:ref}) is equivalent to
\begin{align}
    & \forall i \in \mathcal{N},
    \forall \alpha^\prime_{i} : \Omega \rightarrow \mathcal{A}_{i} \nonumber \\
    & \sum_{\omega \in \Omega} \bm{q}(\omega) u_{i}({\alpha}_i^*(\omega),\bm{\alpha}_{-i}^*(\omega)) \geq \sum_{\omega \in \Omega} \bm{q}(\omega) u_{i}(\alpha^\prime_{i}(\omega), \bm{\alpha}^*_{-i}(\omega))
\end{align}
\begin{flushright}                                      
$\blacksquare$
\end{flushright}
\end{proof}

\newpage

\begin{proposition}
    Let $G$ be a finite non-cooperative game. The distribution $\bm{p}\in\Delta(\mathcal{A})$ is a correlated equilibrium distribution if and only if
    %%%%%%%%%%%%%%%%%%%
    \begin{align}
        & \forall i \in \mathcal{N},
        \forall \beta_i : \mathcal{A}_i \rightarrow \mathcal{A}_i
        \quad
        \sum\limits_{\bm{a} \in \mathcal{A}} \bm{p}(\bm{a}) \left[u_{i}(a_i, \bm{a}_{-i}) - u_{i}(\beta_i(a_i), \bm{a}_{-i}) \right] \geq 0
    \end{align}
    %%%%%%%%%%%%%%%%%%%
\end{proposition}
%%%%%%%%%%%%%%%%%%%%%%%%%%%%
%%%%%%%%%%%%%%%%%%%%%%%%%%%%
\begin{proof}
In this proof, we start by showing (by logical equivalence) the $(\Rightarrow)$ implication of the proposition. We show it by contradiction, \ie if
        %%%%%%%%%%%%%%%%%%%
        \begin{align}
            \exists i \in \mathcal{N},
            \exists \beta^\prime_i : \mathcal{A}_i \rightarrow {\mathcal{A}_i}
            \quad \sum\limits_{\bm{a} \in \mathcal{A}} \bm{p}(\bm{a})
            \left[
                u_{i}(a_i, \bm{a}_{-i}) - u_{i}(\beta_i^\prime(a_i), \bm{a}_{-i}) 
            \right] 
            < 0 
        \end{align}
        %%%%%%%%%%%%%%%%%%%
    then, $\bm{p}$ is not a correlated equilibrium distribution.
    %%%%%%%%%%%%%%%%%%%
    Assume that $\bm{p}$ is a correlated equilibrium distribution and let ${\beta}_i^\prime$ such that 
    %%%%%%%%%%%%%%%%%%%
    \begin{equation}
          \nonumber \\
        \quad \sum\limits_{\bm{a} \in \mathcal{A}} \bm{p}(\bm{a})
        \left[
            u_{i}(a_i, \bm{a}_{-i}) - u_{i}({\beta}^\prime_i(a_i), \bm{a}_{-i}) 
        \right] 
        < 0 
    \end{equation}
    %%%%%%%%%%%%%%%%%%%
    Consider the partitioning $\mathcal{P}_i = \{ P_{b_i}\}_{b_i \in \mathcal{A}_i}$ where $P_{b_i} = \{ \omega \in \Omega : \alpha_i^*(\omega) = b_i \}$ for every $i$. We have,
        \begin{align}
            \forall \bm{a} \in \mathcal{A} \quad \bm{p}_{(x_i,\bm{\alpha}_{-i}^*)}(\bm{a}) = 
            p_{(\beta^\prime_i\circ\alpha_i^*,\bm{\alpha}_{-i}^*)}(\bm{a}) = 
              \bm{z}_{\beta^\prime_i, \bm{p}} (\bm{a})
        \end{align}
    %%%%%%%%%%%%%%%%%%%
    Furthermore, we have,
    %%%%%%%%%%%%%%%%%%%
    \begin{align}
        &
        \sum_{\omega\in\Omega} \bm{q}(\omega) 
        \left[
            u_i(\alpha_i^*(\omega),\bm{\alpha}_{-i}^*) 
            -
            u_i(x_i(\omega),\bm{\alpha}_{-i}^*)
        \right]
        \\
        &= 
        \sum_{\bm{a}\in\mathcal{A}}\bm{p}_{\bm{\alpha}^*}(\bm{a})
        \left[
            u_i(a_i,\bm{a}_{-i}) 
            -
            u_i(\beta^\prime_i(a_i),\bm{a}_{-i})
        \right]\\
        &= 
        \sum_{\bm{a}\in\mathcal{A}}\bm{p}(\bm{a})
        \left[
            u_i(a_i,\bm{a}_{-i}) 
            -
            u_i(\beta^\prime_i(a_i),\bm{a}_{-i})
        \right]
        <0
    \end{align}
    %%%%%%%%%%%%%%%%%%%
    where the last equality follows from the definition of $\bm{p}$ and the inequality is from the assumption on $\beta^\prime_i$.
    Then $\bm{\alpha}^*$ is not a correlated equilibrium implying that $\bm{p}$ is not a correlated equilibrium distribution.\\
    %%%%%%%%%%%%%%%%%%%
    ($\Rightarrow$) Let $\bm{p}$ be a probability distribution such that
    %%%%%%%%%%%%%%%%%%%
    \begin{align}
            \forall i \in \mathcal{N},
            \forall \beta_i : \mathcal{A}_i \rightarrow \mathcal{A}_i \quad 
            \sum\limits_{\bm{a} \in \mathcal{A}} \bm{p}(\bm{a}) 
            \left[u_{i}(a_i, \bm{a}_{-i}) - u_{i}(\beta_i(a_i), \bm{a}_{-i}) \right] \geq 0 
            \label{eq}
    \end{align}
    %%%%%%%%%%%%%%%%%%%
Consider the canonical representation with $d=(\mathcal{A},(\mathcal{P}_i)_{i\in\mathcal{N}},\bm{p})$ such that
$\mathcal{P}_i = \{  P_{a_i} \}_{a_i \in \mathcal{A}_i}$. Let now assume  that each player  uses the strategy $\alpha_i^*:\mathcal{A} \rightarrow  \mathcal{A}_i$ such that $\alpha_i^*(\bm{a})=a_i$ $\forall \bm{a} \in P_{a_i}$. Then the relation (\ref{eq}) becomes:
    %%%%%%%%%%%%%%%%%%%
    \begin{align}
        &\forall i \in \mathcal{N}, 
        \forall \beta_i :  \mathcal{A}_i \rightarrow \mathcal{A}_i \nonumber \\
        & \sum\limits_{a_i \in \mathcal{A}_i} \sum\limits_{\omega \in P_{a_i}} \bm{p}(\omega) 
        \left[
            u_{i}(\alpha^*_i(\omega), \bm{\alpha}^*_{-i}(\omega)) - u_{i}(\beta_i(a_i), \bm{\alpha}^*_{-i}(\omega)) 
        \right] 
        \geq 0
    \end{align}
    %%%%%%%%%%%%%%%%%%%
Let define $\alpha_i^\prime : \mathcal{A} \rightarrow \mathcal{A}_i$ the deviation of player $i$. This means that the player $i$ makes a deviation on different partitions from $\alpha^*_i$. Therefore, any deviation  $\alpha_i^\prime$ can be expressed in terms of this deviation as follows:  $\alpha^\prime_i = \beta_i\circ \alpha^*_i$, where $\beta_i$ is a mapping from $\mathcal{A}_i \rightarrow \mathcal{A}_i$. We have 
\begin{align}
            & \sum\limits_{a_i \in \mathcal{A}_i} \sum\limits_{\omega \in P_{a_i}} \bm{p}(\omega) 
        \left[
            u_{i}(\alpha^*_i(\omega), \bm{\alpha}^*_{-i}(\omega)) - u_{i}(\alpha_i^\prime(w), \bm{\alpha}^*_{-i}(\omega)) 
        \right] \nonumber\\
    & =
  \sum\limits_{a_i \in \mathcal{A}_i} \sum\limits_{\omega \in P_{a_i}} \bm{p}(\omega) 
        \left[
            u_{i}(\alpha^*_i(\omega), \bm{\alpha}^*_{-i}(\omega)) - u_{i}(\beta_i\circ \alpha^*_i(w), \bm{\alpha}^*_{-i}(\omega)) 
        \right] \nonumber\\  
&=  \sum\limits_{\omega \in \Omega} \bm{q}(\omega) 
        \left[
            u_{i}(\alpha^*_i(\omega), \bm{\alpha}^*_{-i}(\omega)) - u_{i}(\beta(a_i), \bm{\alpha}^*_{-i}(\omega)) 
        \right] \geq 0
         \end{align}
Then $\bm{\alpha}^*$ is a correlated equilibrium strategy and the probability distribution it induces $\bm{p}$ is a correlated equilibrium probability distribution.
\begin{flushright}
$\blacksquare$
\end{flushright}
\end{proof}
