# Supplementary material for: Constrained Correlated Equilibria
Source: arXiv:2309.05218 source file (2023-09-12)
Supplement: Supplementary file 3 [file ToBeDiscussed.tex]

%\begin{enumerate}
    %\item \blue{\st{Quantificateurs dans les phrases ou pas ?}} \textcolor{red}{Quantificateurs dans les phrases enlevés}
    %\item \blue{Où est le resultat qui dit que les devices canoniques ne sont plus suffisants dans le cas generique ?} \textcolor{red}{Ajouter le résultat sous forme de remarque dans la Section 4. Trouver l'endroit adéquat pour le mettre.}\\
    %Juste après la définition.
    % \item \textcolor{red}{Proposition \ref{prop:SmallerConstraints} sur la relation entre les distributions contraintes de deux ensembles à discuter}
    %\item \textcolor{red}{Partie explicant les symboles utilisés à remettre?}
    %%%%%%%%%%%%%%%%%%%%%%%%%%%%%%%%%%%%%%%%%%%
    %\item \blue{
    %What about the definition of GNE below where the coupled constraint set $\mathcal{R}$ is used explicitly 
    %%%%%%%%%%%%%%%%%%
    %\begin{definition}[Generalized Nash equilibrium]\label{defn:GNE1}
    %    A generalized Nash equilibrium of a generalized game $G'$ is a strategy profile $\bm{x}^{*}\in\mathcal{R}$ such that, 
    %    \begin{align}
    %        \forall i \in \mathcal{N}, 
    %        \forall x_i \in \mathcal{K}_{i,d}(\bm{x}_{-i}^{*}), 
    %        \quad 
    %        u_i(x^*_i, \bm{x}_{-i}^{*}) \geq u_i(x_i, \bm{x}_{-i}^{*}).
    %    \end{align}
    %\end{definition}}
    %%%%%%%%%%%%%%%%%%
    -%\item \blue{An alternative definition of constrained correlated equilibria can be given without references to generalized Nash equilibria.}
